# Supplementary material for: Learning Representations of Missing Data for Predicting Patient Outcomes
Source: arXiv:1811.04752 source file (2018-11-12)
Supplement: Supplementary file 1 [file patient-outcome-prediction.supplement.pdf]

# Supplement: Learning Representations of Missing Data for Predicting Patient Outcomes

Submission # 832

## Appendix A: Time series data

- Capillary refill rate
- Diastolic blood pressure
- Fraction inspired oxygen
- Glasgow coma scale eye opening
- Glasgow coma scale motor response
- Glasgow coma scale total
- Glasgow coma scale verbal response
- Glucose
- Heart Rate
- Height
- Mean blood pressure
- Oxygen saturation
- Respiratory rate
- Systolic blood pressure
- Temperature
- Weight
- pH

## Appendix B: Note category assignments

Table 1 provides the mapping between the CATEGORY field in the NOTEEVENTS table in MIMIC-III and the 6 types used in this work.

Copyright © 2019, Association for the Advancement of Artificial Intelligence (www.aaai.org). All rights reserved.

Table 1: Note type mapping

| CATEGORY          | Label                      |
|-------------------|----------------------------|
| Case Management   | NOTE OTHER BOW             |
| Consult           | NOTE OTHER BOW             |
| Discharge summary | NOTE DISCHARGE SUMMARY BOW |
| ECG               | NOTE ECG BOW               |
| Echo              | NOTE ECHO BOW              |
| General           | NOTE NURSING BOW           |
| Nursing           | NOTE NURSING BOW           |
| Nursing/other     | NOTE NURSING BOW           |
| Nutrition         | NOTE OTHER BOW             |
| Pharmacy          | NOTE OTHER BOW             |
| Physician         | NOTE NURSING BOW           |
| Radiology         | NOTE RADIOLOGY BOW         |
| Rehab Services    | NOTE OTHER BOW             |
| Respiratory       | NOTE RESPIRATORY BOW       |
| Social Work       | NOTE OTHER BOW             |

## Appendix C: Discharge destinations

Table 2 gives the mapping between the DISCHARGE\_LOCATION field in the ADMISSIONS table in MIMIC-III and the 6 types used in this work.

Table 2: Discharge location mapping

| DISCHARGE_LOCATION        | DD label             |
|---------------------------|----------------------|
| DEAD/EXPIRED              | MORTALITY_INHOSPITAL |
| HOME                      | HOME                 |
| HOME HEALTH CARE          | HOME                 |
| HOME WITH HOME IV PROVIDR | HOME                 |
| HOSPICE-HOME              | HOME                 |
| REHAB/DISTINCT PART HOSP  | REHAB                |
| SNF                       | SNF                  |
| SNF-MEDICAID ONLY CERTIF  | SNF                  |
| LEFT AGAINST MEDICAL ADVI | LEFT                 |
| LONG TERM CARE HOSPITAL   | TRANSFER             |
| DISCH-TRAN TO PSYCH HOSP  | TRANSFER             |
| DISC-TRAN CANCER/CHLDRN H | TRANSFER             |
| OTHER FACILITY            | TRANSFER             |
| SHORT TERM HOSPITAL       | TRANSFER             |
| HOSPICE-MEDICAL FACILITY  | TRANSFER             |
| ICF                       | TRANSFER             |
| DISC-TRAN TO FEDERAL HC   | TRANSFER             |

## Appendix D: Hyperparameter selection

For the results in Section 4 (Experiments) of the main paper, we use an inner three-fold cross-validation on the training set to select the hyperparameters for all linear models. We never use the testing set during training. In particular, the search grids we use are given in Table 3.

Table 3: Hyperparameter search grid

| Logistic regression (MORT and DD) |                               |
|-----------------------------------|-------------------------------|
| Hyperparameter                    | Values                        |
| class weight                      | balanced, no change           |
| regularization type               | l1, l2                        |
| regularization parameter          | 1.0, 0.1, 0.01, 0.001, 0.0001 |

  

| Ridge regression (LOS)   |                                  |
|--------------------------|----------------------------------|
| Hyperparameter           | Values                           |
| regularization parameter | $10^{-6}, 10^{-5} \dots 10^{+7}$ |

Please consult the SCIKIT-LEARN documentation for more details about the hyperparameters.

## Appendix E: Result tables

Tables 4 – 9 give the values shown in Figure 3 of the main text.

## Appendix F: Feature MAE loss

Table 10 gives the normalized MAE loss shown in Figure 4(right) of the main text.

## Appendix G: Feature importance

Figure 1 shows the average contribution of each feature to the final prediction for LOS when training on 100 labeled instances. Specifically, the contribution for each feature on a particular instance is calculated as the sum of the element-wise product of the embedding for the feature with the appropriate coefficients from the learned linear model; we additionally take the absolute value to consider only the magnitude of the contribution.

Figure 2 shows the ratio of the average contributions for each feature when it is observed compared to when it is missing. Larger values indicate that the feature contributes more when it is observed than when it is missing. For example, the embedded Glasgow coma scale motor response feature contributes, on average, about 6 times more to the final prediction when it is observed than when it is missing. In contrast, temperature and pH contribute roughly the same regardless of whether they are observed or not.

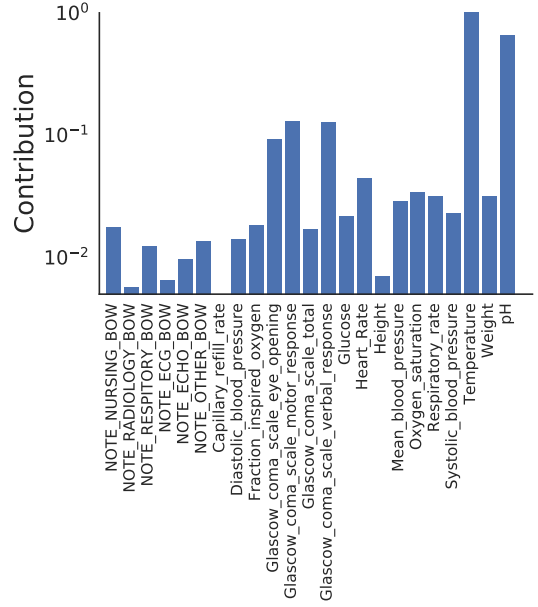

Figure 1: The average contribution of each feature to final predictions across all test instances on LOS when trained with 100 labeled instances.

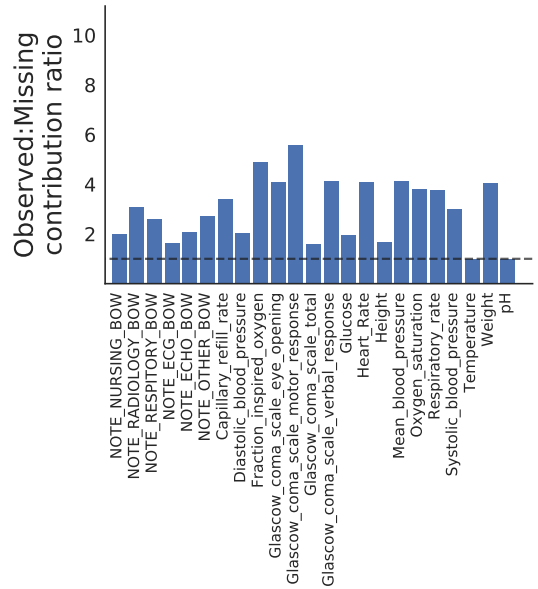

Figure 2: The ratio of the average contribution of each feature to final predictions across all test instances when the feature is observed compared to when it is missing. The dashed line indicates where the ratio is 1, which means the feature contributes equally whether it is observed or not. Higher values indicate that the feature contributes more when it is observed compared to when it is missing.

Table 4: MORT, time series attribute type only

| Number of labeled episodes | COMBINED          | EMBEDDED          | RAW               |
|----------------------------|-------------------|-------------------|-------------------|
| 10                         | $0.556 \pm 0.044$ | $0.605 \pm 0.065$ | $0.551 \pm 0.041$ |
| 20                         | $0.575 \pm 0.047$ | $0.609 \pm 0.057$ | $0.570 \pm 0.066$ |
| 50                         | $0.679 \pm 0.051$ | $0.673 \pm 0.049$ | $0.673 \pm 0.048$ |
| 100                        | $0.745 \pm 0.027$ | $0.708 \pm 0.029$ | $0.745 \pm 0.025$ |
| 500                        | $0.809 \pm 0.010$ | $0.765 \pm 0.010$ | $0.811 \pm 0.011$ |
| 1 000                      | $0.820 \pm 0.007$ | $0.781 \pm 0.007$ | $0.822 \pm 0.006$ |
| 5 000                      | $0.840 \pm 0.003$ | $0.797 \pm 0.005$ | $0.840 \pm 0.005$ |
| 17 869                     | $0.852 \pm 0.000$ | $0.804 \pm 0.000$ | $0.849 \pm 0.000$ |

Table 5: DD, time series attribute type only

| Number of labeled episodes | COMBINED          | EMBEDDED          | RAW               |
|----------------------------|-------------------|-------------------|-------------------|
| 10                         | $0.539 \pm 0.014$ | $0.537 \pm 0.017$ | $0.545 \pm 0.021$ |
| 20                         | $0.557 \pm 0.023$ | $0.549 \pm 0.018$ | $0.560 \pm 0.021$ |
| 50                         | $0.588 \pm 0.016$ | $0.566 \pm 0.016$ | $0.590 \pm 0.015$ |
| 100                        | $0.607 \pm 0.013$ | $0.584 \pm 0.015$ | $0.608 \pm 0.014$ |
| 500                        | $0.645 \pm 0.012$ | $0.618 \pm 0.011$ | $0.644 \pm 0.013$ |
| 1 000                      | $0.658 \pm 0.014$ | $0.634 \pm 0.011$ | $0.656 \pm 0.016$ |
| 5 000                      | $0.688 \pm 0.009$ | $0.659 \pm 0.007$ | $0.688 \pm 0.009$ |
| 17 869                     | $0.709 \pm 0.000$ | $0.673 \pm 0.000$ | $0.707 \pm 0.000$ |

Table 6: LOS, time series attribute type only

| Number of labeled episodes | COMBINED          | EMBEDDED          | RAW               |
|----------------------------|-------------------|-------------------|-------------------|
| 10                         | $4.672 \pm 1.657$ | $3.416 \pm 0.129$ | $5.242 \pm 2.612$ |
| 20                         | $4.714 \pm 1.396$ | $3.416 \pm 0.100$ | $5.143 \pm 1.503$ |
| 50                         | $3.972 \pm 1.443$ | $3.263 \pm 0.073$ | $3.978 \pm 1.443$ |
| 100                        | $3.508 \pm 0.190$ | $3.230 \pm 0.091$ | $3.509 \pm 0.190$ |
| 500                        | $3.334 \pm 0.313$ | $3.166 \pm 0.064$ | $3.399 \pm 0.339$ |
| 1 000                      | $3.202 \pm 0.088$ | $3.131 \pm 0.017$ | $3.239 \pm 0.089$ |
| 5 000                      | $3.001 \pm 0.038$ | $3.053 \pm 0.006$ | $3.034 \pm 0.036$ |
| 17 869                     | $2.956 \pm 0.000$ | $3.028 \pm 0.000$ | $2.985 \pm 0.000$ |

Table 7: MORT, All attribute types

| Number of labeled episodes | COMBINED          | EMBEDDED          | RAW               |
|----------------------------|-------------------|-------------------|-------------------|
| 10                         | $0.659 \pm 0.096$ | $0.587 \pm 0.044$ | $0.665 \pm 0.082$ |
| 20                         | $0.696 \pm 0.053$ | $0.605 \pm 0.061$ | $0.701 \pm 0.066$ |
| 50                         | $0.747 \pm 0.044$ | $0.652 \pm 0.048$ | $0.745 \pm 0.037$ |
| 100                        | $0.769 \pm 0.023$ | $0.690 \pm 0.046$ | $0.766 \pm 0.023$ |
| 500                        | $0.817 \pm 0.008$ | $0.774 \pm 0.012$ | $0.815 \pm 0.010$ |
| 1 000                      | $0.828 \pm 0.005$ | $0.783 \pm 0.009$ | $0.821 \pm 0.007$ |
| 5 000                      | $0.844 \pm 0.003$ | $0.805 \pm 0.004$ | $0.838 \pm 0.005$ |
| 17 869                     | $0.856 \pm 0.000$ | $0.811 \pm 0.000$ | $0.858 \pm 0.000$ |

Table 8: DD, All attribute types

| Number of labeled episodes | COMBINED          | EMBEDDED          | RAW               |
|----------------------------|-------------------|-------------------|-------------------|
| 10                         | $0.574 \pm 0.019$ | $0.563 \pm 0.020$ | $0.573 \pm 0.020$ |
| 20                         | $0.586 \pm 0.019$ | $0.575 \pm 0.023$ | $0.583 \pm 0.016$ |
| 50                         | $0.609 \pm 0.018$ | $0.604 \pm 0.016$ | $0.600 \pm 0.020$ |
| 100                        | $0.620 \pm 0.012$ | $0.617 \pm 0.016$ | $0.611 \pm 0.010$ |
| 500                        | $0.660 \pm 0.014$ | $0.665 \pm 0.008$ | $0.642 \pm 0.018$ |
| 1 000                      | $0.677 \pm 0.014$ | $0.683 \pm 0.015$ | $0.657 \pm 0.016$ |
| 5 000                      | $0.711 \pm 0.011$ | $0.715 \pm 0.005$ | $0.689 \pm 0.012$ |
| 17 869                     | $0.739 \pm 0.000$ | $0.732 \pm 0.000$ | $0.736 \pm 0.000$ |

Table 9: LoS, All attribute types

| Number of labeled episodes | COMBINED          | EMBEDDED          | RAW               |
|----------------------------|-------------------|-------------------|-------------------|
| 10                         | $3.318 \pm 0.109$ | $3.429 \pm 0.106$ | $4.792 \pm 0.055$ |
| 20                         | $3.275 \pm 0.099$ | $3.378 \pm 0.060$ | $4.701 \pm 0.057$ |
| 50                         | $3.215 \pm 0.103$ | $3.316 \pm 0.111$ | $4.584 \pm 0.056$ |
| 100                        | $3.155 \pm 0.053$ | $3.267 \pm 0.088$ | $4.380 \pm 0.077$ |
| 500                        | $3.115 \pm 0.020$ | $3.197 \pm 0.020$ | $3.851 \pm 0.093$ |
| 1 000                      | $3.061 \pm 0.019$ | $3.135 \pm 0.018$ | $3.648 \pm 0.036$ |
| 5 000                      | $2.986 \pm 0.011$ | $3.050 \pm 0.009$ | $3.292 \pm 0.015$ |
| 17 869                     | $2.945 \pm 0.000$ | $3.024 \pm 0.000$ | $3.162 \pm 0.000$ |

Table 10: MAE loss shown in Figure 4(right) of the main text.

| Attribute                          | Embedded MAE loss | Raw MAE loss |
|------------------------------------|-------------------|--------------|
| Capillary refill rate              | -0.023301         | 0.580816     |
| Diastolic blood pressure           | -0.156282         | -0.064640    |
| ETHNICITY                          | 0.002419          | 0.057705     |
| Fraction inspired oxygen           | 0.022698          | 0.136004     |
| Glasgow coma scale eye opening     | -0.307864         | 0.019429     |
| Glasgow coma scale motor response  | -0.304350         | 0.020988     |
| Glasgow coma scale total           | -0.044169         | -0.130732    |
| Glasgow coma scale verbal response | -0.307864         | 0.019429     |
| Glucose                            | -0.094687         | 0.027558     |
| Heart Rate                         | -0.156282         | -0.064640    |
| Height                             | 0.006909          | 0.100878     |
| MARITAL STATUS                     | -0.070432         | -0.106718    |
| Mean blood pressure                | -0.156282         | -0.064640    |
| NOTE DISCHARGE SUMMARY BOW         | 0.233990          | 0.284654     |
| NOTE ECG BOW                       | -0.025505         | -0.021364    |
| NOTE ECHO BOW                      | -0.018772         | 0.017316     |
| NOTE NURSING BOW                   | -0.016769         | -0.120556    |
| NOTE OTHER BOW                     | 0.001341          | 0.021422     |
| NOTE RADIOLOGY BOW                 | 0.004466          | 0.041344     |
| NOTE RESPITORY BOW                 | 0.014245          | 0.028457     |
| Oxygen saturation                  | -0.092130         | 0.091678     |
| Respiratory rate                   | -0.150736         | -0.050517    |
| Systolic blood pressure            | -0.156282         | -0.064640    |
| Temperature                        | -0.101287         | -0.194498    |
| Weight                             | -0.005509         | 0.073845     |
| pH                                 | -0.001081         | 0.091238     |
